# Supplementary material for: Dynamic interfaces for contact-time control of colloidal interactions
Source: arXiv:2303.08880 ancillary file (2023-03-15)
Supplement: Supplementary file 1 [file Colloids_Contact_Time_PRL_Supplement.pdf]

# Dynamic interfaces for contact-time control of colloidal interactions

## Supplemental Material

Yaxin Xu\*, Kyu Hwan Choi\*, Sachit G. Nagella, Sho C. Takatori

## Contents

|          |                                                                           |           |
|----------|---------------------------------------------------------------------------|-----------|
| <b>1</b> | <b>Theoretical framework and simulations</b>                              | <b>2</b>  |
| 1.1      | Theory development . . . . .                                              | 2         |
| 1.1.1    | Smoluchowski Equation . . . . .                                           | 2         |
| 1.1.2    | Particle Interactions . . . . .                                           | 2         |
| 1.1.3    | Colloid Approach Speed . . . . .                                          | 3         |
| 1.2      | Brownian Dynamics Simulations . . . . .                                   | 3         |
| 1.2.1    | Particle interactions . . . . .                                           | 4         |
| 1.2.2    | Approach protocol . . . . .                                               | 4         |
| <b>2</b> | <b>Experimental methods</b>                                               | <b>5</b>  |
| 2.1      | Optical laser tweezers setup . . . . .                                    | 5         |
| 2.2      | Preparation of observation cell . . . . .                                 | 5         |
| 2.3      | Preparation of F-actin grafted colloid . . . . .                          | 6         |
| 2.3.1    | Small unilamellar vesicle (SUV) synthesis . . . . .                       | 6         |
| 2.3.2    | Formation of supported lipid bilayer (SLB) on silica beads . . . . .      | 6         |
| 2.3.3    | Grafting F-actin on SLB . . . . .                                         | 7         |
| 2.4      | Characterization of fabricated particles . . . . .                        | 7         |
| 2.4.1    | Characterization of grafting actin density . . . . .                      | 7         |
| 2.4.2    | Characterization of grafting actin length . . . . .                       | 8         |
| 2.5      | Force measurement . . . . .                                               | 8         |
| 2.5.1    | Calibration of trap stiffness . . . . .                                   | 9         |
| 2.5.2    | Defining equilibrium state . . . . .                                      | 10        |
| <b>3</b> | <b>Fluid-mediated effects between colloidal particles</b>                 | <b>11</b> |
| 3.1      | Equations of motion . . . . .                                             | 11        |
| 3.2      | Application of the lubrication approximation . . . . .                    | 13        |
| 3.2.1    | Bare particles . . . . .                                                  | 13        |
| 3.2.2    | Effect of end-grafted polymer chains on hydrodynamic resistance . . . . . | 14        |
| <b>4</b> | <b>Supplemental Movies</b>                                                | <b>15</b> |

# 1 Theoretical framework and simulations

## 1.1 Theory development

In this section, we model nonequilibrium distribution of polymers with laterally-mobile grafting sites on the surface of two colloids when they are brought into contact. We consider their probability distribution through a Smoluchowski equation and model the relaxation of interfacial polymers via monomer diffusion. Finally, we calculate the instantaneous, polymer-mediated force exerted between the colloidal pair at close contact.

### 1.1.1 Smoluchowski Equation

We consider two colloids of size  $d_c$  in a Newtonian fluid with viscosity  $\eta$ , where one is located at the origin and the other at relative position  $\mathbf{r}$ . The colloidal surfaces are each coated by semi-rigid polymer brushes of polymerization  $M$  and surface density  $n_\rho$  that are able to diffuse laterally across the surfaces. The conditional probability distribution  $P_N(\mathbf{h}_1, \dots, \mathbf{h}_N, t; \mathbf{r})$  of finding  $N$  monomer particles at relative position  $\mathbf{h}_1, \dots, \mathbf{h}_N$  for a given colloidal separation  $\mathbf{r}$  satisfies the time and space-dependent Smoluchowski equation:

$$\frac{\partial P_N}{\partial t} + \sum_{i=1}^N \nabla_i \cdot \mathbf{j}_i = 0 \quad (1)$$

with the flux of  $\alpha$  given by:

$$\mathbf{j}_i = - \sum_{j=1}^N \mathbf{D}_{ij} P_N \cdot \nabla_j \left( \ln P_N + \frac{V_{\text{tot}}}{k_B T} \right) \quad (2)$$

where  $V_{\text{tot}}(\mathbf{h}_1, \dots, \mathbf{h}_N; \mathbf{r})$  is the total potential energy, and  $\mathbf{D}_{ij}$  is the diffusivity. In the absence of hydrodynamic interactions, the monomer diffusivity follows the Stokes-Einstein-Sutherland relation  $\mathbf{D}_{ij} = \mathbf{I}_{ij} k_B T / \zeta_i$ .

Assuming the polymers are semi-dilute, Eq. 1 is integrated over  $N-1$  monomer degrees of freedom to recover Eq.(1) - (2) in the main text. The governing equation satisfies monomer mass conservation  $\int \rho d\mathbf{h} = 1$  and no flux at colloid-monomer contact. Note that the total potential energy is replaced with a mean-field potential  $V$  which accounts for interactions between the monomer and the two colloids. We next discuss the polymer brush model used to approximate  $V$ .

### 1.1.2 Particle Interactions

The equilibrium monomer number density at position  $z$  above the surface in a polymer brush is approximated as a smooth, gaussian profile:

$$n_{\text{eq}}(z) \approx n_\rho e^{-(z^2 - h_0^2)/h_0^2} \quad (3)$$

where  $h_0$  is the height at which monomer density decays to zero. Note that  $h_0 \sim 9\mu\text{m}$  is set using the simulations.

From the equilibrium monomer distribution, the mean field pair potential between the monomer and the reference colloid can be defined as

$$V_{\text{single colloid}}(z) = -k_B T \ln(n_{\text{eq}}(z)/n_{\text{eq}}(0)). \quad (4)$$

We now approximate the potential of the monomer around two colloidal particles by summing the Boltzmann distributions of the monomers around each colloid at equilibrium:

$$V = -\ln(n_{\text{eq}}(||\mathbf{h}||) + n_{\text{eq}}(||\mathbf{h} - \mathbf{r}||)) \quad (5)$$

Under this definition, we recover the equilibrium distributions of polymer density around both colloids when in the limit of non-overlapping brushes,  $H \gg 2h_0 + 2d_c$ . We further note that the intrinsic hard sphere collisions between colloids and monomers  $V_{\text{HS}} = \Theta(||\mathbf{h}||) + \Theta(||\mathbf{h} - \mathbf{r}||)$  do not explicitly enter into the potential but is instead incorporated as the no flux boundaries discussed previously.

Given the pair interaction potential  $V$ , the effective polymer mediated force on the reference colloid directly follows as  $\langle \mathbf{F} \rangle = n_\rho M \int \rho \nabla_{\mathbf{r}} V d\mathbf{h} + n_\rho M \oint \rho \mathbf{n}_1 dS_1$ , where the first term is the elastic force and the second term represents the osmotic force resulting from increased hard sphere collisions at contact. We define  $F = \mathbf{F} \cdot \mathbf{e}_x$  as the force magnitude along the colloidal line of centers. At equilibrium, this polymer mediated force is weaker than the potential derived by Dolan and Edwards for compressed polymer brushes whose grafting sites are immobile [1] because (1) our model neglects forces resulting from chain compression and (2) laterally-mobile polymers can exclude from the contact interface.

### 1.1.3 Colloid Approach Speed

Up until now, we have defined an evolution equation for the monomer when colloidal particles are fixed in space, governed by thermal diffusion and inter-particle forces. In order to consider the nonequilibrium dynamics as the colloidal system relaxes, we require an appropriate nonequilibrium starting configuration of monomer density  $\rho$ . We hypothesize the starting monomer configuration is modulated by the speed at which colloids are brought into contact. The interfacial concentration of monomers on opposing colloidal surfaces should increase proportionally to the speed at which colloids are compressed,  $\rho \sim \text{Pe} \rho_{\text{eq}}$ , where we have defined a Péclet number  $\text{Pe} = v\sigma/D_\rho$  for the relative timescale for colloids to compress the polymer brushes versus the diffusive motion of the monomers. Note that  $\rho(\mathbf{h}, t = 0|\mathbf{r})$  is normalized to satisfy mass conservation over all  $\mathbf{h}$ .

## 1.2 Brownian Dynamics Simulations

Two colloids of size  $d_c = 4\sigma$  in a solvent of viscosity  $\eta$  are coated by standard Kremer-Grest bead-spring polymers [2]. The simulation length scale is  $\sigma = 1\mu\text{m}$  and the dimensions of the periodic simulation box are  $L_y = L_z = 33\sigma$ ,  $L_x = 65\sigma$ .

We coarse-grain polymer segments into beads of diameter  $d_\rho = 0.8\mu\text{m}$  with 17 beads per chain. Results shown in Fig. 1 of the main text are obtained for a surface coverage  $\phi = n_\rho(d_\rho^2/4d_c^2) = 0.15$ . To compare with experimental results in Fig. 3, we choose surface coverages of  $\phi = 0.15 - 0.43$  to match actin surface-densities of  $\phi_{\text{F-actin}} = \pi(d_{\text{F-actin}}/2)^2\rho_{\text{F-actin}} \approx 0.11 - 0.46$  where the F-actin monomer size is  $d_{\text{F-actin}} = 7\text{nm}$  (see Supp. Video 3). For all simulations, we choose a time step size  $\Delta t = (2 \times 10^{-5})(\sigma^2/D_\rho)$  and sample the simulation every  $10^3$  time steps. We average over 20 realizations to obtain representative statistics of the nonequilibrium approach and relaxation processes. Simulations are performed using HOOMD-Blue, a GPU-accelerated simulation package.

Recognizing that the momentum relaxation timescale is much faster than the diffusive timescale in our system, the trajectory of each polymer bead in time  $t$  follows the overdamped Langevin equation of motion:

$$\frac{\Delta \mathbf{x}_i}{\Delta t} = \left( \underbrace{\mathbf{F}_i^{\text{P}}}_{\text{interactions}} + \underbrace{\mathbf{F}_i^{\text{R}}}_{\text{Brownian}} \right) / \zeta \quad (6)$$

where  $\mathbf{x}_i$  is the position of particle  $i$ , and  $\zeta = 3\pi\eta d_\rho$  is the drag coefficient. Note that the Stokes-Einstein-Sutherland diffusivity of the polymer bead is defined as  $D_\rho = k_{\text{B}}T/\zeta$ . In accordance with fluctuation dissipation, the implicit solvent induces a stochastic force satisfying  $\langle \mathbf{F}_i^{\text{B}} \rangle = 0$  and  $\langle \mathbf{F}_i^{\text{B}}(0)\mathbf{F}_i^{\text{B}}(t) \rangle = 2k_{\text{B}}T(\zeta_i)\mathbf{I}\delta(t)$ . Unlike the polymer beads which undergo stochastic motion, the colloidal cores either move with deterministic motion towards each other at some fixed speed (during the approach step) or are fixed in space and cannot undergo any translation (during the relaxation step).

### 1.2.1 Particle interactions

All non-bonded particle pairs interact through a Weeks-Chandler-Anderson (WCA) hard sphere-like potential with parameters  $\epsilon = \alpha = k_{\text{B}}T$ . Adjacent polymer beads in a chain to interact through a Finite-Extensible-Nonlinear-Elastic (FENE) potential with equilibrium bond parameter  $r_0 = 1.5\sigma$  and attraction strength  $k_{\text{FENE}} = 30k_{\text{B}}T$ . Additionally, we employ a harmonic potential penalizing the angle  $\theta$  between two adjacent bonds,  $V_{\text{ang}} = (1 - \cos(\theta - \pi))l_\rho/\sigma$  where the persistence length is  $l_\rho = 13\sigma$ . To graft polymers onto the colloidal surface, we constrain the bead corresponding to the polymer grafting site between two, concentric spherical walls, such that the grafting site may still translate laterally but cannot detach from the surface.

### 1.2.2 Approach protocol

At the start of the simulation, polymer chains are first allowed to equilibrate at an initial colloidal separation  $H = 30\sigma$  where the brushes are non-overlapping. During the approach process, colloid and polymer bead positions are incrementally updated to move closer by  $\Delta H_{\text{incrm}} = 0.005\sigma - 0.08\sigma$  every  $\Delta t_{\text{incrm}} = 10^2 - 10^3$  time steps to bring colloids together to different separation distances

$30\sigma < H < d_c$  (see Supp. video 1).  $\Delta H$  and  $t_{\text{incrim}}$  are adjusted to fix the colloid approach velocity  $v$  (see Supp. video 2). Finally, polymers are allowed to relax from their nonequilibrium configurations for  $10^6 - 10^7$  time steps as colloids are held fixed at separation  $H$ . During the approach and relaxation steps, the polymer-mediated force on the colloids  $\langle F \rangle = \sum_i F_i^P$  is computed every  $10^2 - 10^3$  time steps.

## 2 Experimental methods

The main text already contains a description of our experimental methods; in this section, we provide additional experimental detail on optical tweezer set-up and particle fabrication.

### 2.1 Optical laser tweezers setup

Colloidal particles were manipulated using optical laser tweezers (Tweez 305, Aresis Ltd, Slovenia) with a continuous infrared laser (wavelength: 1064nm, maximum power: 5W) equipped on an inverted fluorescence microscope (Ti2-Eclipse, Nikon) using oil immersion Apo 100x objective lens (Numerical Aperture(NA) 1.45, Nikon). As an excitation light source, Lumencor SpectraX Multi-Line LED Light Source (Lumencor, Inc) was used at two different wavelengths (488nm and 647nm). A multi-wave emission filter (515/30, 680/42; Semrock, IDEX Health and Science) spectrally filtered the fluorescent lights. Videos were acquired by CMOS camera, (Photometrics Prime 95, Teledyne Photometrics) with 100 frames per second(fps) for force measurements, and 15 fps for other videos. CMOS and microscope were operated using Micromanager 1.4 on ImageJ. Trap positions were regulated by importing time-trajectory Matlab scripts to Tweez 305 software with 25mW/particle as a set value, not a measured power on the objective.

### 2.2 Preparation of observation cell

The observation cell described in main text Fig. 2a was constructed on a  $170 \pm 5 \mu\text{m}$  thickness high precision coverslip (Marienfeld) as a glass substrate, with a 5mm thick Polydimethylsiloxane (PDMS, Sylgard 184, Dow), with a  $\phi 6\text{mm}$  hole as a wall on the glass substrate. To prevent colloids from sticking to the glass substrate, the observation cell was coated with Poly(l-lysine)-graft-5k poly(ethylene glycol) (PLL-*g*-PEG, Nanosoft BIotechnology LCC.)[3]. The passivation coating on the glass was treated by spreading  $30 \mu\text{L}$  of 0.1 mg/mL PLL-*g*-PEG aqueous solution to piranha-cleaned glasses. After 30 min, the treatment solution was discarded from the cell. The remaining unbound PLL-*g*-PEG was washed by pipetting fresh Milli-Q (MQ) water vigorously. This washing process was repeated more than 5 times using fresh MQ water for every washing cycle.

| Sample name | Lipids          |          |          |                  |
|-------------|-----------------|----------|----------|------------------|
|             | DGS-NTA(Ni) [%] | DOPC [%] | DPPC [%] | DOPE-Atto488 [%] |
| 10% Ni-NTA  | 10              | 89       | -        | 1                |
| 1% Ni-NTA   | 1               | 98       | -        | 1                |
| SLB only    | 0               | 99       | -        | 1                |
| DPPC        | 10              | -        | 89       | 1                |

Table 1: Compositions of lipid for each SUV sample

## 2.3 Preparation of F-actin grafted colloid

Colloids coated with surface-mobile polymer were fabricated by grafting filamentous actin (F-actin) on supported lipid bilayer (SLB) coated silica microbeads (Fig. 2b-d, Fig. 4a-b).  $4\mu\text{m}$  diameter silica microbeads,  $d_c = 4\mu\text{m}$ , were purchased from Bangs Laboratories and cleaned by piranha solution, a 3:2 mixture of sulfuric acid and hydrogen peroxide, through bath sonication for 30 min. Then, the cleaned bead slurry was washed with MQ water by re-dispersing and sedimenting using a centrifuge,  $10,000 \times g$  for 3min. Chemicals used in this experiment were purchased from Sigma-Aldrich if there are no notations.

### 2.3.1 Small unilamellar vesicle (SUV) synthesis

To modify the surface properties (i.e. actin density, and mobility), small unilamellar vesicles (SUVs) were designed for each experiment. We perform tip-sonication to form SUVs from the lipid solution [4]. Lipids 1,2-dioleoyl-sn-glycero-3-phos-phocholine (DOPC), 1,2-dipalmitoyl-sn-glycero-3-phosphocholine (DPPC), and 1,2-dioleoyl-sn-glycero-3-[(N-(5-amino-1- carboxypentyl)iminodiacetic acid)succinyl] (DGS-NTA(Ni), Ni-NTA), were purchased from Avanti Polar Lipids. A fluorescence lipid, Atto 488-1,2-dioleoyl-sn-glycero-3-phosphoethanolamine (DOPE-Atto488), was purchased from ATTO-TEC GmbH. Lipid solutions were mixed at specific molecular ratios in a disposable glass culture tube. All residual solvents were evaporated from the solution using a vacuum chamber for 30min. After 30min, the dried lipid film was rehydrated in MQ water to  $0.2\text{mg/mL}$  for 10min. Before tip sonication, the rehydrated solution was vortexed and transferred to a  $1.5\text{mL}$  tube. The solution was then sonicated for 3min (1s/2s, on/off cycle) with a 20% of the maximum power of a tip-sonicator (Branson SFX250 Sonifier). Finally, 10x MOPS buffer was added to balance the osmotic pressure across the SLB, with a final concentration of 50mM MOPS pH 7.4 and 100mM NaCl. The compositions of SUVs for corresponding samples are described in Table 1.

### 2.3.2 Formation of supported lipid bilayer (SLB) on silica beads

The SLB was formed on glass beads by incubating  $10\mu\text{L}$  of silica particle solution and an excess amount ( $50\mu\text{L}$ ) of composition-controlled SUVs solution for 15 minutes at room temperature. To fabricate DPPC-containing SLB, we melt DPPC lipids in a convection oven at  $40^\circ\text{C}$  in a convection oven for 2min. Free

SUVs were washed with HEPES buffer (50mM HEPES pH 7.4, 100mM NaCl) by gently removing the supernatant and adding fresh HEPES buffer without disturbing the lipid-coated particle sediment. During the last two washes, F-buffer was used instead of HEPES to exchange the buffer conditions for the next step. The F-buffer composition is 50mM Tris pH 7.5, 2mM MgCl<sub>2</sub>, 0.2mM CaCl<sub>2</sub>, 25mM KCl, 0.5mM adenosine 5'-triphosphate (ATP), and 1mM dithiothreitol (DTT).

### 2.3.3 Grafting F-actin on SLB

We polymerized F-actin directly on the SLB-coated silica bead described in main text (Fig. 2b, Fig. 4b). SLB-coated beads, 100nM 6x-histidine tagged gelsolin (6x-His-Gel, HPG6, Cytoskeleton, Inc.), 20 $\mu$ M monomeric actin (G-actin, purified by following the method with modification [5]), 18 $\mu$ M phalloidin(Invitrogen), and 2 $\mu$ M 647-dyed phalloidin(Alexa Fluor Plus 647 Phalloidin, Invitrogen) were added to F-buffer in the following steps. We first mix 6x-His-Gel with SLB-coated particles and then wait for 2 min for Histidine-Nickel binding to occur. The Histidine of 6x-His-Gel is directly anchored to the Ni<sup>+</sup>-site of DGS-NTA(Ni) on the SLB, and Gelsolin grabs onto the end of F-actin. After 45min, the polymerization reaction was quenched by diluting the solution concentration 20 times using HEPES buffer. We gently pipetted to mix the solution because F-actin is fragile to breaking. After waiting 15min for particle sedimentation, unreacted reactants were washed without resuspending the particle sediment by discarding the supernatant through gentle pipetting. Fresh HEPES buffer was then injected. The actin-grafted beads were used after repeating the washing process more than 5 times.

## 2.4 Characterization of fabricated particles

### 2.4.1 Characterization of grafting actin density

To obtain the surface density of F-actin on the SLB at various DGS-NTA(Ni) concentrations, we compare against standard fluorescence beads (Quantum Alexa Fluor 647 MESF, Bangs Laboratories), which have precise sizes and known numbers of fluorescent dyes on the surface. The dye densities on reference beads are calculated by dividing the number of dyes by the surface area,  $\rho_{\text{dye, ref}} = \frac{N_{\text{dye}}}{4\pi R^2}$ . To construct a calibration line, the standard beads were dispersed in the 8-well chambered coverglass system (170 $\pm$ 5 $\mu$ m, Cellvis) and imaged with constant camera values, 16-bit depth, 500ms of exposure time, and 10% of maximum power (wavelength centered at: 647nm).

From the images, the maximum brightness of the particles was plotted against surface number density of the dye (Fig. S1). We perform a linear regression,  $I = \alpha \cdot \rho_{\text{dye}} + I_0$ , using 5 different standard beads, where  $I$  is an intensity of fluorescence signal,  $\alpha$  is the slope of the linear fit,  $\rho_{\text{dye}}$  is a number density of the dye [dyes/ $\mu\text{m}^2$ ], and  $I_0$  is the background noise of the fluorescence image. Actin-grafted colloids were prepared with a logarithmic scale of DGS-NTA(Ni)

concentration in the SLB (0.01, 0.1, 1, and 10%). The fluorescence intensity of F-actin grafting samples was measured from 647 nm existing fluorescence images with the same conditions as standard beads. Number densities of the dye were then converted to F-actin grafting densities by multiplying the molar ratio of total phalloidin to dyed phalloidin,  $N_{\text{total}}/N_{\text{dyed}} = 10$ , since binding one G-actin to the filament requires one phalloidin for stabilization[6].

Surface grafting densities on reference beads were  $\rho_{\text{dye, ref}}$ ; 0-3,441 dyes/ $\mu\text{m}^2$  (Fig. S1). The linear regression parameters are,  $\alpha = 4.6\mu\text{m}^2$ ,  $I_0 = 135.5$ . The brightness of fabricated actin grafting beads was also measured with 5 different logarithmic scale DGS-NTA(Ni) concentrations. From the measured intensities, the dye densities were derived using the following equation,  $\rho_{\text{F-actin}} = \frac{N_{\text{total}}}{N_{\text{dyed}}} \rho_{\text{dye}} = 10(I - I_0)/\alpha$ . So, the number densities of F-actin are  $\rho_{\text{F-actin, 10\%}} = 12,293 \pm 1,030$  filaments/ $\mu\text{m}^2$ ,  $\rho_{\text{F-actin, 1\%}} = 3,211 \pm 568$  filaments/ $\mu\text{m}^2$ . We hypothesize one reason why the actin surface density does not increase linearly with DGS-NTA(Ni) concentration is because short F-actin filaments tend to crowd the SLB surface at higher concentrations, preventing additional anchoring.

#### 2.4.2 Characterization of grafting actin length

The length of grafting F-actin on the 10% Ni-NTA membrane was measured from high-contrast fluorescence images. Images and videos were acquired by 50ms of exposure time, 10% of 647nm excitation laser powers. The range of F-actin length was roughly 2-20 $\mu\text{m}$  with a mean of 5 $\mu\text{m}$ . (Fig. S 2, and Supp. Video 4) We note that the dimness of the long filaments is attributed to rapid photo-bleaching by the laser. The DPPC membrane has a different length distribution of 2-5 $\mu\text{m}$  with a mean of 3 $\mu\text{m}$ . (Fig. 4a, and Supp. Video 7)

### 2.5 Force measurement

As outlined in the main text, force measurements between two colloids were conducted over an approach process followed by relaxation. (Fig. 2e, Supp. Video 5, 6) The two traps are initialized at long separation, 35 $\mu\text{m}$ , where opposing F-actin filaments are non-interacting. The left particle is held at a stationary trapping position to measure forces while the right particle moves towards the stationary colloid with a constant speed during the approach process ( $t < 0$ ). At  $t = 0$ , the moving trap has held a position and immediately started a relaxation process. Time-position data was imported from Matlab to Tweeze 305 software. We measured dynamic interactions for 5 different approach speeds, 0.5, 1, 2, 5, and 10 $\mu\text{m/s}$ . Forces were calculated from the following equation,  $F = \kappa_t \cdot dx$ , where  $\kappa_t$  is a trap stiffness of the optical trap, and  $dx$  is a particle displacement from the trapping focus. During force measurements, photo-bleaching was suppressed by adding an oxygen scavenger into the medium. The oxygen-removing solution consists of 600nM of glucose oxidase from *Aspergillus niger*, 30nM of catalase from bovine liver, and 10mM glucose.

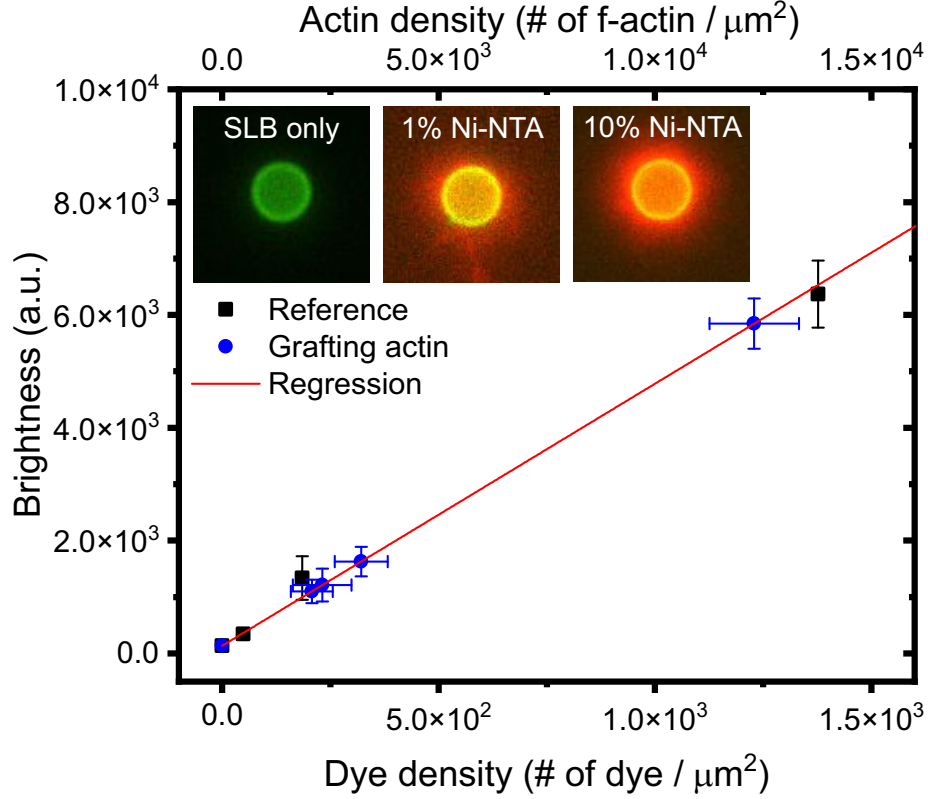

Figure 1: Brightness changing in the dye density of standard particles and surface grafted actin. Inset images are corresponding pictures that have 0, 1, and 10% DGS-NTA(Ni) lipids on SLB. Red and green colors in the inset images are represented by F-actin and SLB respectively. Black squares are representing the fluorescence intensity of reference beads. The red line is the linear regression fit of the standard beads. The blue circles are measured data of the fabricated actin grafted colloids.

### 2.5.1 Calibration of trap stiffness

To compute the trap stiffness  $\kappa_t$ , we note that F-actin surface concentration influenced the thermal vibrations of the stationary trap. To account for this, we construct a probability distribution from more than 4,000 positions of the trapped bead. The radial displacement,  $dr$ , from the laser focus was then fit with Boltzmann distribution,  $P(dr) = \frac{\kappa_t}{2\pi} \exp(-\kappa_t dr^2 / 2k_B T)$ . From the probability distribution curve, we obtained a range of trap stiffness,  $\kappa_t : 0.5 - 0.7 pN/\mu\text{m}$ .

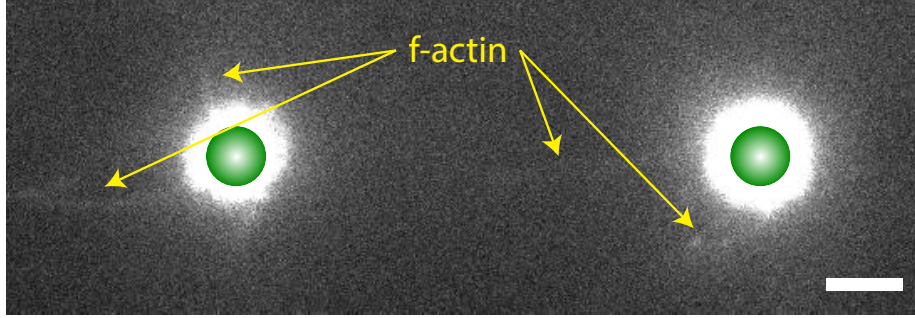

Figure 2: Fluorescence image of long actin filaments grafted on the 1% DGS-NTA(Ni) SLB by increasing brightness and contrast. The scale bar is 5  $\mu\text{m}$ . See also Supp. Video 4.

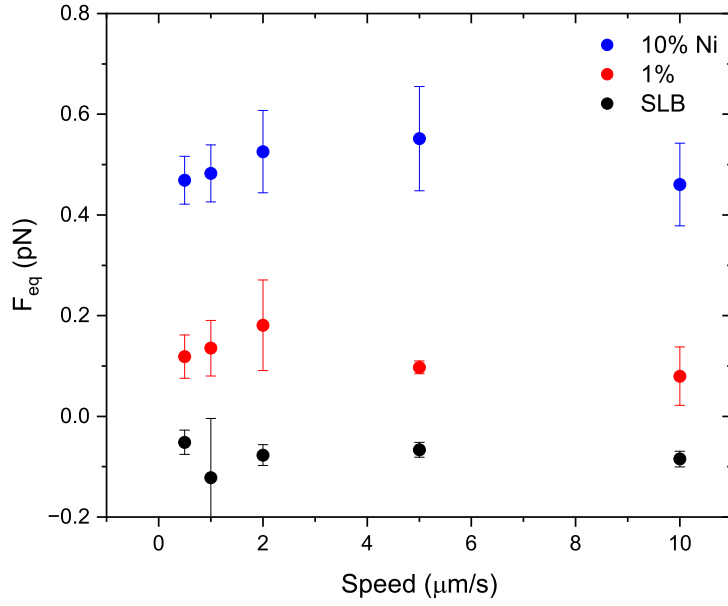

Figure 3: Measured equilibrium forces,  $F_{\text{eq}}$ , after finishing relaxation processes,  $t > \tau_{\text{R}}$ . 10% Ni-NTA, 1% Ni-NTA, and SLB only are corresponding to blue, red, and black circles. The particle having the same grafting density makes similar equilibrium forces, not depending on the approach process.

### 2.5.2 Defining equilibrium state

To characterize the force relaxation as the system approaches equilibrium, we define a relaxation time  $\tau_{\text{R}}$  for the peak force to decay 90% toward the equi-

librium value (Fig. 2f). In other words,  $F(t = \tau_R) = F_{\max} - 0.9(F_{\max} - F_{\text{eq}})$ , where  $F_{\max}$  is a maximum peak force at  $t = 0$ , and  $F_{\text{eq}}$  is the equilibrium force at long times,  $t \gg \tau_R$ . The equilibrium force is calculated by averaging over the range  $15\text{sec} < t < 20\text{sec}$  when the force has fully decayed. We observe that the equilibrium force is independent of approach speed and increases for higher F-actin surface densities (Fig. S3). We note that SLB-only colloids have negative forces because of van-der Waals type attractions.

### 3 Fluid-mediated effects between colloidal particles

Colloidal interactions are known to be heavily influenced by fluid effects in many systems. We now delve into a more thorough consideration of hydrodynamic interactions.

#### 3.1 Equations of motion

The early-time interfacial relaxation depends on the nonequilibrium protocol used to bring the colloidal beads to their final separation. That is, the nonequilibrium driving force, given by the moving colloid's velocity  $v$ , determines the initial force distribution, from which it relaxes with a timescale  $\tau_R$  that we measured.

For now, we will concern ourselves with the details of the dynamic force measurement during the particle approach. The measured trapping forces,  $F^{\text{ext}}(t)$ , represent the instantaneous force required to maintain the equilibrium position of the stationary bead. However, as the stiffness parameter  $\kappa_t$  is finite, the stationary bead will exhibit displacement, as the moving bead induces solvent-mediated hydrodynamic flows. In the case of bare beads, the transmission of solvent-mediated friction forces,  $F^{\text{H}}$ , throughout the fluid of density  $\rho$  and viscosity  $\eta$ , disturbs the stationary particle from the laser focus. Grafting a polymeric layer on the lipid bilayer introduces additional interactions,  $F^{\rho}$ . Taken together, we can write a generalized force balance for a colloidal particle of mass  $m$  that accounts for these effects.

$$m \frac{d\mathbf{v}}{dt} = \mathbf{F}^{\text{ext}} + \mathbf{F}^{\text{H}} + \mathbf{F}^{\rho}. \quad (7)$$

For simplicity, we will neglect the stochastic forces which arise from the bombardment of solvent molecules.

In the following, we will focus on the details of the hydrodynamic force. The motion of any translating colloid displaces solvent at a rate  $\sim d_c^2 v$  on length-scales comparable the bead diameter  $d_c$ . This displacement is accompanied by inertial ( $\sim \rho d_c^2 v^2$ ) and drag forces ( $\sim \eta d_c v$ ), and their ratio, known as the Reynolds number,  $Re = \rho d_c v / 2\eta$ , describes their relative importance. Owing to the small length scales of the system ( $\sim \mu\text{m}$ ),  $Re \ll 1$ , we may neglect inertial effects. Consequently, we may ignore the left-hand-side of (7), imposing the

constraint that all forces must sum to zero. By a similar argument, rotational inertia is negligible, and the sum of torques on the particles is also zero. To determine the hydrodynamic force in this friction-dominated limit, one must solve the Stokes equations in the incompressible solvent

$$\nabla^2 \mathbf{u} - \nabla p = \mathbf{f}, \quad (8)$$

$$\nabla \cdot \mathbf{u} = 0, \quad (9)$$

where the local velocity field  $\mathbf{u}$  is driven by any combination of moving boundaries (e.g., the beads in motion), dynamic pressure gradients  $\nabla p$ , or body forces  $\mathbf{f}$ . For now, we will ignore any external body forces so that  $\mathbf{f} = \mathbf{0}$ .

As the Stokes equations are linear in velocity, so, too, are the hydrodynamic forces. That is,  $F^H \sim \zeta v$ , where  $\zeta$  is a drag coefficient. For an isolated, translating sphere, this relationship is Stokes' law,  $F^H = -3\pi\eta d_c v$ . However, the form for  $\zeta$  becomes increasingly complicated in the presence of nearby particles, as their rigid boundaries interfere with the long-ranged flow disturbances induced by any one bead. Due to this interference, we must account for additional forces that are also linear with the particle velocity. Then, we may consider the total hydrodynamic force and torque on each particle,  $\hat{\mathbf{F}}^H = (\mathbf{F}_1^H, \mathbf{F}_2^H, \dots, \mathbf{T}_1^H, \mathbf{T}_2^H, \dots)$ . Here, the subscripts denote particle index. Exploiting linearity and superposition of the forces and torques in low- $Re$  flows, we can express the total hydrodynamic force as the linear combination of all fluid-mediated resistances to particle translation and rotation, using the matrix-vector product

$$\hat{\mathbf{F}}^H = -\mathcal{R} \cdot \hat{\mathbf{v}}. \quad (10)$$

The components of matrix  $\mathcal{R}$  are the pairwise resistance tensors that account for the hydrodynamic interactions parallel and perpendicular to the line-of-centers, whose functional forms are tabulated [7]. Because of the lack of time-dependence in (9), the “transient” flow field induced by a moving particle possesses no memory. As a result, the hydrodynamic resistances contained in  $\mathcal{R}$  only depend on the instantaneous particle configurations.

For bare particles,  $\hat{\mathbf{F}}^H = -\hat{\mathbf{F}}^{\text{ext}}$ , so any force measurements given by OT satisfy the relationship (again, ignoring stochastic forces),

$$\hat{\mathbf{F}}^{\text{ext}} = \mathcal{R} \cdot \hat{\mathbf{v}}. \quad (11)$$

Knowledge of the forces enables solving linear system (11) for the particle velocities and vice-versa. For two beads without external torques, (11) becomes

$$\begin{pmatrix} \mathbf{F}_1^{\text{ext}} \\ \mathbf{F}_2^{\text{ext}} \\ \mathbf{0} \\ \mathbf{0} \end{pmatrix} = \begin{pmatrix} \mathbf{R}_{11}^{\text{FU}} & \mathbf{R}_{12}^{\text{FU}} & \mathbf{R}_{11}^{\text{F}\omega} & \mathbf{R}_{12}^{\text{F}\omega} \\ \mathbf{R}_{21}^{\text{FU}} & \mathbf{R}_{22}^{\text{FU}} & \mathbf{R}_{12}^{\text{F}\omega} & \mathbf{R}_{22}^{\text{F}\omega} \\ \mathbf{R}_{11}^{\text{TU}} & \mathbf{R}_{12}^{\text{TU}} & \mathbf{R}_{11}^{\text{T}\omega} & \mathbf{R}_{12}^{\text{T}\omega} \\ \mathbf{R}_{21}^{\text{TU}} & \mathbf{R}_{22}^{\text{TU}} & \mathbf{R}_{12}^{\text{T}\omega} & \mathbf{R}_{22}^{\text{T}\omega} \end{pmatrix} \begin{pmatrix} \mathbf{v}_1 \\ \mathbf{v}_2 \\ \boldsymbol{\omega}_1 \\ \boldsymbol{\omega}_2 \end{pmatrix}, \quad (12)$$

where the superscripts indicate the coupling, and subscripts the particle pair. Thus, the measured force on the stationary colloid  $\mathbf{F}_1^{\text{ext}}$  linearly depends

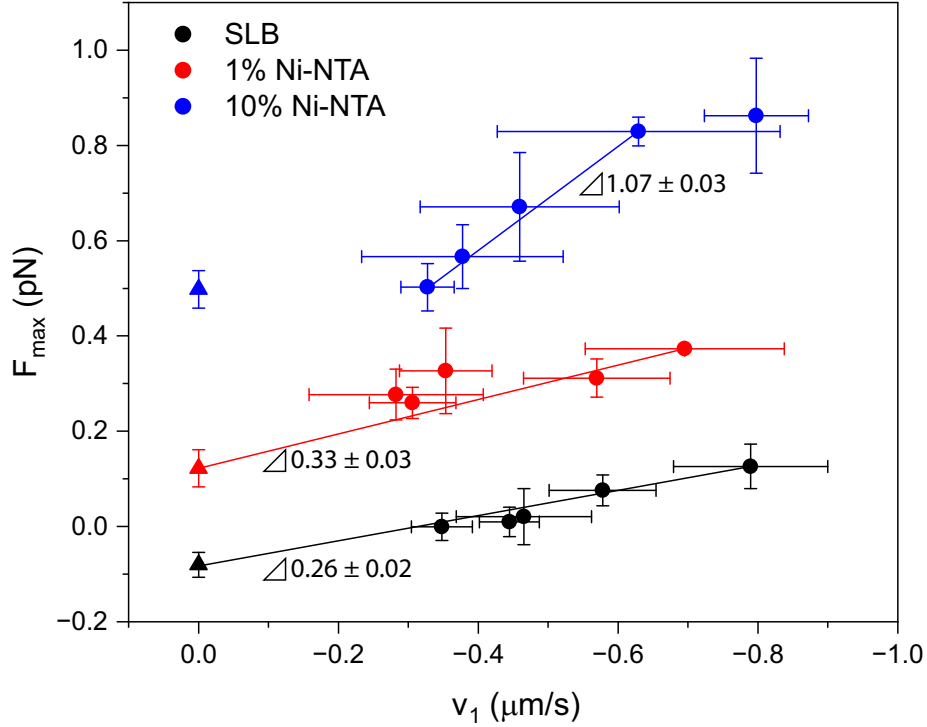

Figure 4: Maximum trapping forces on the stationary bead generally scale linearly with the instantaneous velocity  $v_1$ , upon closest approach with the moving particle. The instantaneous bead velocities  $v_1$  were determined from each approach velocity used. Forces at  $v_1 = 0$  are the equilibrium interactions between the particles, taken to be the “quasi-static” limit.

on the translational and rotational velocities of the particles. While (12) appears cumbersome, we can consider the limit in which the particles are in close contact.

## 3.2 Application of the lubrication approximation

### 3.2.1 Bare particles

Now, we will demonstrate that the lubrication approximation is sufficient to predict the scale of our force measurements and its dependence on bead velocity. As shown in Fig. 2 of the main text, the moving bead is brought to the stationary particle at a fixed speed until they reach close contact, corresponding to the measurement  $F_{\text{max}}$ . Focusing on bare particles (“SLB only”), the observed maximum in the force is due to hydrodynamics. As the moving bead approaches the stationary particle, it diverts fluid from the interface and consequently experiences viscous drag. When the interfacial gap thickness is much smaller than the particle radius, the pressure difference between the interface and the sur-

rounding medium “far away” increases significantly to expel fluid from the thin film (i.e., the lubricant). Reynolds (1886) solved (9) in the asymptotic limit of a sphere approaching a planar surface at fixed speed. Equivalently, as in our system, we consider the two particles asymptotically approaching the symmetry half-plane between them, i.e.  $\epsilon \equiv (H - d_c)/d_c \ll 1$ , given that  $H$  is the center-to-center separation. Reynolds determined that the hydrodynamic force scaled sensitively with the aspect ratio, such that  $F^H = 3\pi\eta d_c v \epsilon^{-1}$ .

To apply this result to our data and estimate the hydrodynamic drag on the bare particles, we compared the measurements of the maximum force with the instantaneous velocities of the stationary bead, which we computed from the displacement time-trajectories (Fig. S4). Upon closest approach ( $H - d_c \approx 400\text{nm}$ ), the bare stationary particle moves away from the incoming bead due to the increasing hydrodynamic force (see Supp. Video 7). Then, the moving particle suddenly stops and is held in place, and the stationary bead reverses its motion. Still, the repulsive hydrodynamic force points opposite to that of the potential gradient.

This momentary configuration of the beads is convenient to analyze, as the moving particle is now held in place ( $\mathbf{v}_2 = \mathbf{0}$ ) while the stationary particle moves towards the laser focus at an instantaneous velocity  $\mathbf{v}_1$ . From (10), there are additional resistances due to the coupling between the forces and rotations. Generally, a torque-free particle can simply rotate in response to local shearing by the fluid flow, effectively reducing the translational resistance. Yet, in the thin-gap limit,  $\|\mathbf{R}_{F\omega}\| \sim \ln(\epsilon^{-1})$ , providing a quantitative correction to the purely squeezing motion (parallel to line-of-centers) between two bare surfaces [8]. Therefore, we expect the force response on the stationary colloid to behave as

$$\mathbf{F}_1^{\text{ext}} = \mathbf{R}_{11}^{\text{FU}} \cdot \mathbf{v}_1 + O(\ln(\epsilon^{-1})), \quad (13)$$

where  $\|\mathbf{R}_{11}^{\text{FU}}\| \sim 3\pi\eta d_c \epsilon^{-1} \approx 0.39\text{pN}/\mu\text{m/s}$ . We find that slope of the force-velocity data, the hydrodynamic resistance, for the bare particles is to within order of magnitude of the Reynolds prediction. Because the theoretical result overestimates the measurement, we attribute the difference to ignoring particle rotations.

### 3.2.2 Effect of end-grafted polymer chains on hydrodynamic resistance

We believe that the addition of actin on the lipid bilayer surface increases the hydrodynamic resistance to the solvent flow during bead approach (Fig. S4). Increasing the surface density of the actin layer corresponded to a larger interparticle separation at closest approach of the moving bead. As such, while the measured maximum forces were taken at different interparticle distances, the steeper slope for the highest actin density (10% Ni-NTA) at greater separations indicates a greater hydrodynamic resistance. We rationalize this enhancement in the observed resistance by considering the increased viscous dissipation inside the polymer layer. Whereas the solvent flows unimpeded out of the interfacial

volume for two bare beads, introducing the polymer layers sets up a locally porous medium that inhibits fluid flow. We emphasize that because the peak force measurements were not taken at small gap separations, straightforward application of lubrication theory will not demonstrate agreement with the experimental data. However, should the gap separation be consistent with the compression of the end-grafted actin layers, we may refer to existing theories for a prediction of the hydrodynamic force.

Viscous flows through porous media are typically modeled using the Brinkman equation, a variation of the Stokes equations wherein  $\mathbf{f} = \frac{\eta}{K}\mathbf{v}$ .  $K$  is the permeability of the medium. Fredrickson and Pincus (1991) applied a lubrication-type analysis of the Brinkman equation to determine the hydrodynamic force between two grafted polymer surfaces. Arguing that the local structure within thin-gap of overlapping polymer layers resembles that of a semi-dilute polymer solution, they determined the permeability in terms of the equilibrium mean separation between chains and its dependence on gap separation (i.e.,  $\epsilon$ ). From this, the enhanced hydrodynamic force now scales as  $F^H \sim \epsilon^{-\frac{1}{2}}$ , a stronger dependence on the geometric aspect ratio than in the Reynolds result. This change in the scaling reflects the greater required pressure gradient to squeeze fluid through the polymeric mesh at the contact interface. Such an analysis would be valid on the nonequilibrium process timescales which are slower than that of actin reorganization, so that the grafted layer behaves as a "static" mesh whose structure is unperturbed by fluid flow. Otherwise, one would have to self-consistently solve the Stokes equations with a model for the body force  $\mathbf{f} = \mathbf{f}(\rho(\mathbf{h}|H, \mathbf{v}))$  that couples to the polymer dynamics [9, 10].

## 4 Supplemental Movies

Below, we describe the Supplemental Movies associated with this manuscript. All time stamps corresponds to hours:minutes:seconds. All scale bars represent  $5\mu\text{m}$ .

**S1.** Brownian Dynamics simulations of two colloids (blue) coated by coarse-grained polymers (red) with surface density  $n_\rho\sigma^2 = 0.15$ , laterally-mobile grafting sites (gray). Polymers relax after being brought together to varying separations  $H$  instantaneously quickly.

**S2.** Brownian Dynamics simulations of polymer-coated colloids with surface density  $n_\rho\sigma^2 = 0.15$  brought to a close separation at varying approach speeds  $v$ .

**S3.** Brownian Dynamics simulations of polymer-coated colloids brought to a close separation at a fixed approach speed and varying surface densities  $n_\rho$ .

**S4.** Fluorescence movie of F-actin on two SLB-coated colloids containing 1% Ni-NTA. F-actin length varies from short brushes ( $h_0 \approx 2\mu\text{m}$ ) to very long filaments ( $h_0 \approx 20\mu\text{m}$ ).

**S5.** Fluorescence movie of SLB channel for F-actin grafted colloids during the approach ( $t < 0$ ) and relaxation ( $t > 0$ ) processes, where right colloid translates with fixed speed ( $10\mu\text{m/s}$ ). The red dot is the laser focus position on the

reference colloid.

**S6.** Fluorescence movie of F-actin during approach and relaxation processes for 1% Ni-NTA SLB-coated colloids.

**S7.** Fluorescence movie of hydrodynamic interactions between SLB-only beads. (x0.2 speed of original speed)

**S8.** Fluorescence movie of rigid, protruding F-actin bundles on the non-diffusive SLB-coated colloid containing 10% Ni-NTA and 89% DPPC.

## Bibliography

- [1] A. K. Dolan and S. F. Edwards. *Proceedings of the Royal Society of London. A. Mathematical and Physical Sciences* 337.1611 (Apr. 1974), pp. 509–516.
- [2] K. Kremer and G. S. Grest. *The Journal of Chemical Physics* 92.8 (1990), pp. 5057–5086.
- [3] H. Turlier et al. *Nature physics* 12.5 (2016), pp. 513–519.
- [4] J. M. Barakat and S. C. Takatori. *Physical Review E* 107.1 (2023), p. 014601.
- [5] J. A. Spudich and S. Watt. *Journal of biological chemistry* 246.15 (1971), pp. 4866–4871.
- [6] P. Dancker et al. *Biochimica et Biophysica Acta (BBA)-Protein Structure* 400.2 (1975), pp. 407–414.
- [7] D. J. Jeffrey and Y. Onishi. *Journal of Fluid Mechanics* 139 (Feb. 1984), pp. 261–290.
- [8] M. E. O’Neill and K. Stewartson. *Journal of Fluid Mechanics* 27.4 (1967), pp. 705–724.
- [9] P. S. Doyle, E. S. Shaqfeh, and A. P. Gast. *Macromolecules* 31.16 (1998), pp. 5474–5486.
- [10] P. S. Doyle, E. S. G. Shaqfeh, and A. P. Gast. *Phys. Rev. Lett.* 78 (6 Feb. 1997), pp. 1182–1185.
